# Supplementary material for: MagicAnimate: Temporally Consistent Human Image Animation using Diffusion Model
Source: arXiv:2311.16498 source file (2023-11-27)
Supplement: Supplementary file 1 [file supplementary.tex]

\clearpage
\setcounter{page}{1}
\maketitlesupplementary
